# Supplementary material for: Mitigating Privacy-Utility Trade-off in Decentralized Federated Learning via $f$-Differential Privacy
Source: arXiv:2510.19934 source file (2025-10-22)
Supplement: Supplementary file 1 [file Appendix_V1.tex]

\section{Privacy amplification by iteration}
\begin{lemma}
    Let $X_{t}$ and $X_{t}'$ respectively be the output of ${\rm CNI}(X_0, \{\phi_{k}\}+{k \in [t]}, \{\cN(0, \sigma^2 \Ib_p)\}{k \in [t]}, \cK)$ and ${\rm CNI}(X_0, \{\phi_{k}^{'}\}+{k \in [t]}, \{\cN(0, \sigma^2 \Ib_p)\}{k \in [t]}, \cK)$ such that each $\phi_{k}, \phi_{k}'$ is $c-$Lipschitz and $\|\phi_{k} - \phi_{k}^{'}\|_{\infty} \leq s_{k}$ for all $k \in [t]$. Then for any intermediate time $\tau$ and shift parameters $\lambda_{\tau + 1}, \cdots, \lambda_{t} \in [0,1]$ with $\lambda_{t} = 1$, 
    \begin{align*}
        T(X_{t}, X_{t}') \geq G\left( \frac{1}{\sigma} \sqrt{\sum_{k = \tau+1}^{t} a_{k}^2} \right)
    \end{align*}
    where $a_{k+1} = \lambda_{k+1} (c z_{k} + s_{k+1})$, $z_{k+1} = (1 - \lambda_{k+1}) (c z_{k} + s_{k+1})$, and $\|X_{\tau} - X_{\tau}'\| \leq z_{\tau}$. 
\end{lemma}

When $s_k = 0$ for all $k > K$, we have the following lemma.
\begin{lemma}
    Given $D > 0$, the optimal value of 
    \begin{align*}
        \min \sum_{k=\tau+1}^{t} a_{k}^2
    \end{align*}
    subject to 
    \begin{align*}
        a_{k+1} = \lambda_{k+1} z_{k} \geq 0, \quad z_{k+1} = (1 - \lambda_{k+1}) z_{k} \geq 0, \quad z_{\tau} = D, \quad z_{t} = 0, \quad 1 \geq \lambda_{k} \geq 0.
    \end{align*}
    is $\frac{D^2}{t - K}$ and the value is minimized when $\tau = K$. 
\end{lemma}
\begin{proof}
Notice
\begin{align*}
    z_{t} + a_{t} =\ & z_{t-1}
    \\
    z_{t} + a_{t} + a_{t-1} =\ & z_{t-1} + a_{t-1} = z_{t-2}
    \\
    &\cdots
    \\
    z_{t} + a_{t} + a_{t-1} + \cdots + a_{\tau+1} =\ & z_{\tau} = D
\end{align*}
This further implies that 
\begin{align*}
    a_{t} + \cdots + a_{\tau+1} &= z_{\tau} = D
\end{align*}
By Cauchy-Schwarz inequality, we have
\begin{align*}
    \sum_{k=\tau+1}^{t} a_{k}^2 \geq \frac{\left( a_{t} + \cdots + a_{\tau+1} \right)^2}{t - \tau} = \frac{D^2}{t - \tau} \geq \frac{D^2}{t - K}.
\end{align*}

\end{proof}

\subsection{Refined analysis for federated learning}
\begin{lemma}
    When $\tau = 0$, given $0 < c < 1$, the optimal value of 
    \begin{align*}
        \min \sum_{k=1}^{t} a_{k}^2
    \end{align*}
    subject to 
    \begin{gather*}
        a_{k+1} = \lambda_{k+1} (cz_{k}+s_{k+1}) \geq 0, \quad z_{k+1} = (1 - \lambda_{k+1}) (cz_{k}+ s_{k+1}) \geq 0, \quad z_{0} = 0, \quad z_{t} = 0,                \\ \quad 0 \leq \lambda_{k} \leq 1,\quad
        s_{k} \equiv \Delta, \hbox{ for } 0\leq k \leq K, \quad \hbox{ and } s_k=0,\hbox{ for } K+1\leq k \leq KT,
    \end{gather*}
    is $\frac{1+ c}{1 - c} \cdot \frac{(1 - c^{K})^2}{1 - c^{2t}} s^2$.
\end{lemma}

\begin{proof}
Note that 
\begin{align*}
    z_{t} + \sum_{k=\tau + 1}^t c^{t - k} a_k =\ & z_0 + \sum_{k=\tau + 1}^t c^{t - k} s_{k}
    \\
    \sum_{k=\tau + 1}^t c^{t - k} a_k =\ & \frac{1 - c^{K}}{1-c} s
\end{align*}
By the Cauchy-Schwarz inequality, we have
\begin{align*}
    \sum_{k=\tau+1}^t a_k^2 \geq \frac{\left( \sum_{k=\tau + 1}^t c^{t - k} a_k \right)^2}{\sum_{k=\tau + 1}^t c^{2(t - k)}} = \frac{1+ c}{1 - c} \cdot \frac{(1 - c^{K})^2}{1 - c^{2t}} s^2.
\end{align*}
\end{proof}

\begin{lemma}[Lemma C.12 in \cite{Bok2024shifted}] For $s \geq 0$ and $0 \leq p \leq 1$, let
    \begin{align*} R(s, \sigma, p) = \inf \{T(VW + Z, VW' + Z): &\ V \sim \text{Ber}(p), \norm{W}, \norm{W'} \leq s, Z \sim \cN(0, \sigma^2 I_d)\}\, 
    \end{align*}
    where the infimum is taken pointwise and is over independent $V, W, W', Z$. Then $R(s, \sigma, p) \geq C_p(G(\frac{2s}{\sigma}))$.
\end{lemma}

\begin{theorem}\label{thm:sgd-sc-gen} Consider $m$-strongly convex, $M$-smooth loss functions with gradient sensitivity $L$. Then for any $\eta \in (0, 2/M)$, $t > K$, Noisy SGD is $f$-DP where
\begin{align*}
    f =\ & G \left( \frac{2\sqrt{2}c z_{tK-1}}{\eta \sigma} \right) \otimes \bigotimes_{k=1}^{tK-1}C_{p_k}\left( G \left(\frac{2a_k}{\eta \sigma} \right) \right) 
\end{align*}
for any sequence such that $z_0 = 0$, $0 < \lambda_{k} < 1$ and $\{z_{k}, a_{k}, s_{k}\}$ is given by
    \begin{align*}
        z_{k+1} =\ & \max\{ cz_k , (1-\lambda_{k+1})(cz_k + s_{k})\}
        \\
        a_{k+1} =\ & \lambda_{k+1} \left( c z_{k} + s_{k} \right)
        \\
        s_{k} =\ & \max\{ \|\phi_{S_{k}} - \psi_{S_{k}}\|_{\infty}, \|\phi'_{S'_{k}} - \psi_{S'_{k}}\|_{\infty} \}. 
    \end{align*}
and $c = \max\{|1 - \eta m|, |1 - \eta M|\}$, $s_{k} = 0$, $p_{k} = 0$ for any $k > K$.
\end{theorem}
\begin{proof}
    The iterates of Noisy SGD with respect to $\{f_i\}_{i \in [n]}$ and $\{f'_i\}_{i \in [n]}$ are
    \begin{align*}
        X_{k+1} &= \Pi_{\cK}(\psi_{S_k}(X_k) + V_k(\phi_{S_k} - \psi_{S_k})(X_k) + Z_{k+1}) \\
        X'_{k+1} &= \Pi_{\cK}(\psi_{S'_k}(X'_k) + V'_k(\phi'_{S'_k} - \psi_{S'_k})(X'_k) + Z'_{k+1})\,,
    \end{align*}
    where $Z_{k+1}, Z'_{k+1} \sim \cN(0, \eta^2 \sigma^2 I_d)$. Now consider shifted interpolated processes defined as
    \begin{align*}
        \widetilde{X}_{k+1} &= \Pi_{\cK}(\psi_{S_k}(\widetilde{X}_k) + \lambda_{k+1}V_k(\phi_{S_k}(X_k) - \psi_{S_k}(\widetilde{X}_k)) + Z_{k+1}) \\
        \widetilde{X}'_{k+1} &= \Pi_{\cK}(\psi_{S'_k}(\widetilde{X}'_k) + \lambda_{k+1}V'_k(\phi'_{S'_k}(X'_k) - \psi_{S'_k}(\widetilde{X}'_k)) + Z'_{k+1})\,,
    \end{align*}
    with $\widetilde{X}_0 = \widetilde{X}'_0 = X_0$
    \begin{lemma} \label{eqn:interpolation_trade}
    The trade-off function between $\widetilde{X}_{t-1}$ and  $\widetilde{X}'_{t-1}$ is given by
        \begin{align*}
            T(\widetilde{X}_{t-1}, \widetilde{X}'_{t-1}) \geq \bigotimes_{k=1}^{t-1} C_{p_k} \left( G\left( \frac{2 a_{k}}{\eta \sigma} \right) \right)
        \end{align*}
    where $\{z_{k}, a_{k}, s_{k}\}$ is given by
    \begin{align*}
        z_{k+1} =\ & \max\{ cz_k , (1-\lambda_{k+1})(cz_k + s_{k})\}
        \\
        a_{k+1} =\ & \lambda_{k+1} \left( c z_{k} + s_{k} \right)
        \\
        s_{k} =\ & \max\{ \|\phi_{S_{k}} - \psi_{S_{k}}\|_{\infty}, \|\phi'_{S'_{k}} - \psi_{S'_{k}}\|_{\infty} \}. 
    \end{align*}
    \end{lemma}
    To relate this with $T(X_t, X'_t)$, note that there is no choice of $\lambda_t$ that yields $\widetilde{X}_t = X_t$. 
    Instead, we can proceed as follows: write down the corresponding update (before taking the projection) as
      \begin{align*}
        &\;\psi_{S_{t-1}}(X_{t-1}) + V_{t-1}(\phi_{S_{t-1}} - \psi_{S_{t-1}})(X_{t-1}) + Z_t
        \\ =&\; \psi_{S_{t-1}}(\widetilde{X}_{t-1}) + \psi_{S_{t-1}}(X_{t-1}) - \psi_{S_{t-1}}(\widetilde{X}_{t-1}) + Z^{(1)}_t + V_{t-1}(\phi_{S_{t-1}} - \psi_{S_{t-1}})(X_{t-1}) + Z^{(2)}_t
    \end{align*}
    where $Z^{(1)}_t, Z^{(2)}_t \sim \cN(0, \frac{\eta^2 \sigma^2}{2}I_d)$\footnote{In general, we can split the noise into $Z_t = Z^{(1)}_t + Z^{(2)}_t$ where $Z^{(1)}_t \sim \cN(0, \frac{\eta^2 \sigma^2}{\alpha^2}I_d)$ and $Z^{(2)}_t \sim \cN(0, \frac{\eta^2 \sigma^2}{\beta^2}I_d)$ are independent and $1/\alpha^2 + 1/\beta^2 = 1$. Then the part $G(\frac{2\sqrt{2}cz_{t-1}}{\eta \sigma}) \otimes C_{b/n}(G(\frac{2\sqrt{2} L}{b \sigma}))$ in the last line of the proof is replaced with $G(\frac{2\alpha cz_{t-1}}{\eta \sigma}) \otimes C_{b/n}(G(\frac{2\beta L}{b \sigma}))$.} are independent, $\psi_{S_{t-1}}(X_{t-1}) - \psi_{S_{t-1}}(\widetilde{X}_{t-1})$ is bounded by $cz_{t-1}$ and $(\phi_{S_{t-1}} - \psi_{S_{t-1}})(X_{t-1})$ is bounded by $\frac{\eta L}{b}$. Then
    \begin{align*}
        &T(X_t, X'_t) \\
        &\geq T((\widetilde{X}_{t-1}, S_{t-1}, \psi_{S_{t-1}}(X_{t-1}) - \psi_{S_{t-1}}(\widetilde{X}_{t-1}) + Z^{(1)}_t), (\widetilde{X}'_{t-1}, S'_{t-1}, \psi_{S'_{t-1}}(X'_{t-1}) - \psi_{S'_{t-1}}(\widetilde{X}'_{t-1}) + Z^{(1)'}_t)) \\
        &\quad\otimes R\left( s_{t-1}, \frac{\eta \sigma}{\sqrt{2}}, b/n \right) \\
        &\geq T((\widetilde{X}_{t-1}, S_{t-1}), (\widetilde{X}'_{t-1}, S'_{t-1})) \otimes R \left(cz_{t-1}, \frac{\eta \sigma}{\sqrt{2}}, 1 \right) \otimes R\left( s_{t-1}, \frac{\eta \sigma}{\sqrt{2}}, b/n \right) \\
        &\geq T(\widetilde{X}_{t-1}, \widetilde{X}'_{t-1}) \otimes G \left(\frac{2\sqrt{2}cz_{t-1}}{\eta \sigma} \right)\,.
    \end{align*}
\end{proof}

\begin{proof}[Proof of Lemma \ref{eqn:interpolation_trade}]
    $\{z_k\}_{0 \leq k \leq t-1}$ and $\{a_k\}_{0 \leq k \leq t-1}$ satisfies $z_0 = 0, a_0 = \frac{\sqrt{2} \eta L}{b}$ and $z_{k+1} = \max\{ cz_k , (1-\lambda_{k+1})(cz_k + s_{k})\}$ for all $k \geq 0$. 
    Inductively $\norm{\widetilde{X}_k - X_k} \leq z_k$ for all $k$ from
    \[\norm{\widetilde{X}_{k+1} - X_{k+1}} \leq \begin{cases} \norm{\psi_{S_k}(X_k) - \psi_{S_k}(\widetilde{X}_k)} \leq cz_k & V_k = 0 \\ \norm{(1-\lambda_{k+1})(\phi_{S_k}(X_k) - \psi_{S_k}(\widetilde{X}_k))} \leq (1-\lambda_{k+1})(cz_k + s_{k}) & V_k = 1 \end{cases}
    \]
    where 
    \begin{align*}
        \max\{ \|\phi_{S_{k}} - \psi_{S_{k}}\|_{\infty}, \|\phi'_{S'_{k}} - \psi_{S'_{k}}\|_{\infty} \} \leq s_{k}.
    \end{align*}
    and 
    \begin{align*}
        &\norm{\lambda_{k+1}(\phi_{S_k}(X_k) - \psi_{S_k}(\widetilde{X}_k))}
        \\
        \leq\ & \norm{\lambda_{k+1}(\phi_{S_k}(X_k) - \phi_{S_k}(\widetilde{X}_k))} + \norm{\lambda_{k+1}(\phi_{S_k}(\widetilde{X}_k) - \psi_{S_k}(\widetilde{X}_k))} 
        \\
        \leq\ & \lambda_{k+1} \left( c z_{k} + s_{k} \right) = a_{k+1} 
    \end{align*}
    Similar results hold for $\{X'_k\}$. 
    Therefore, 
    \begin{align*}
        &T \left( \widetilde{X}_{t-1}, \widetilde{X}'_{t-1} \right)
        \\
        \geq\ & T\left(\psi_{S_{t-2}}(\widetilde{X}_{t-2}) + \lambda_{t-1}V_{t-2}(\phi_{S_{t-2}}(X_{t-2}) - \psi_{S_{t-2}}(\widetilde{X}_{t-2})) + Z_{t-1}, \right.
        \\
        &\qquad \qquad \qquad \left.\psi_{S'_{t-2}}(\widetilde{X}'_{t-2}) + \lambda_{t-1}V'_{t-2}(\phi'_{S'_{t-2}}(X'_{t-2}) - \psi_{S'_{t-2}}(\widetilde{X}'_{t-2})) + Z'_{t-1} \right)
        \\
        =\ & T \left( (\widetilde{X}_{t-2}, S_{t-2}, \lambda_{t-1}V_{t-2}(\phi'_{S'_{t-2}}(X'_{t-2}) - \psi_{S'_{t-2}}(\widetilde{X}'_{t-2})) + Z_{t-1}), \right.
        \\
        &\qquad \qquad \qquad \qquad \left. (\widetilde{X}'_{t-2}, S'_{t-2}, \lambda_{t-1}V'_{t-2}(\phi'_{S'_{t-2}}(X'_{t-2}) - \psi_{S'_{t-2}}(\widetilde{X}'_{t-2}))  + Z'_{t-1}) \right)
        \\
        \geq\ & T \left( \widetilde{X}_{t-2}, \widetilde{X}'_{t-2} \right) \otimes T \left( \lambda_{t-1}V_{t-2}(\phi'_{S'_{t-2}}(X'_{t-2}) - \psi_{S'_{t-2}}(\widetilde{X}'_{t-2})) + Z_{t-1},\right.
        \\
        &\qquad \qquad \qquad \qquad \qquad \qquad \qquad \left. \lambda_{t-1}V'_{t-2}(\phi'_{S'_{t-2}}(X'_{t-2}) - \psi_{S'_{t-2}}(\widetilde{X}'_{t-2}))  + Z'_{t-1} \right)
        \\
        \geq\ & \bigotimes_{k=1}^{t-1} C_{p_k} \left( G\left( \frac{2 a_{k}}{\eta \sigma} \right) \right)
    \end{align*}
\end{proof}

When $s_{k} = 0$, $p_{k} = 0$ for any $k > K$, the following holds.
\begin{align*}
    f =\ & G \left( \frac{2\sqrt{2}c z_{tK-1}}{\eta \sigma} \right) \otimes \bigotimes_{k=1}^{tK-1}C_{p_k}\left( G \left(\frac{2a_k}{\eta \sigma} \right) \right) 
    \\
    =\ & G \left( \frac{2\sqrt{2}c z_{tK-1}}{\eta \sigma} \right) \otimes \bigotimes_{k=1}^{K}C_{p_k}\left( G \left(\frac{2a_k}{\eta \sigma} \right) \right) \otimes \bigotimes_{k=K+1}^{Kt-1}G \left(\frac{2}{\eta \sigma} \sqrt{\sum_{k=K}^{tK-1} a_{k}^2} \right)
    \\
    =\ & G \left( \frac{2\sqrt{2}c^{(t-1)K} z_{K}}{\eta \sigma} \right) \otimes \bigotimes_{k=1}^{K}C_{p_k}\left( G \left(\frac{2a_k}{\eta \sigma} \right) \right)
\end{align*}

\section{Iteration}

To bound $f_{ij}^t$, we employ recently developed privacy amplification by iteration using $f$-DP (Bok et al., 2024).
Due to the local updates, the privacy amplification skill can now be decomposed into two parts: the iterations on node $i$ and the iterations after the model is sent out from node $i$ until it reaches $j$.

For the iterations on node $i$, we consider $f^{0} := T(\theta_{K,0},\theta_{K,0}')$ for $\theta_{K,0}'$ being the model trained by $D'$ such that $D'\sim_i D.$

\begin{lemma}
% \label{lemma:iteration}
    Suppose that the loss functions $\ell_i$ on the node $i$ is $M_1$-strongly convex, $M_2$-smooth, then it holds $f_{ij}^t \geq G_{\mu_t}$ with 
    \begin{align*}
        \mu_t = \sqrt{\frac{1+ c}{1 - c} \cdot \frac{(1 - c^{K})^2}{1 - c^{2Kt}}}\frac{\Delta}{b\sigma},
    \end{align*}
    where $c = \max\left\{|1 - \eta M_1|, |1 - \eta M_2| \right\}$ and $b$ is the mini-batch size.
\end{lemma}

\begin{lemma}
    For $t>1$, we have $f_{ij}^t \geq G_\mu$ with  $\mu \geq \min\left\{\frac{D}{\sigma\sqrt{K(t-1)}},\frac{\sqrt{K}\Delta}{\sigma\sqrt{t}} \right\}.$
\end{lemma}
\begin{proof}
    The theorem is a straightforward application of Theorem C.3 in \cite{Bok2024shifted} by taking $a_{k} \equiv \frac{D}{t(K-1)},$ $z_k = \frac{D(tK-k)}{t(K-1)},$ and $\lambda_k = \frac{1}{tK-k+1}.$
\end{proof}

% \clearpage
% \noindent
% \cite{Cyffers2024differentially}:
% \begin{align*}
%     \epsilon^{\rm single} \leq \sum_{i=1}^{T} \PP\left( \text{u $\mapsto$ v after i steps}\right) \cdot \beta(i)
% \end{align*}
% \noindent
% Hitting Time:
% \begin{align*}
%     \epsilon^{\rm single} \leq\ & \sum_{t=1}^{T} \sum_{s=1}^{t} \PP\left( \text{u $\mapsto$ v after t steps, exit time = s}\right) \cdot \beta(s)
%     \\
%     =\ & \sum_{s=1}^{T} \sum_{t=s}^{T} \PP\left( \text{u $\mapsto$ v after t steps, exit time = s}\right) \cdot \beta(s)
%     \\
%     =\ & \sum_{s=1}^{T} \sum_{t=s}^{T} \PP\left( \text{u $\mapsto$ u after s steps}\right) \PP\left( \text{u $\mapsto$ v after t-s steps without attain u}\right) \cdot \beta(s)
%     \\
%     =\ & \sum_{t=1}^{T} \sum_{s + k = t} \PP\left( \text{u $\mapsto$ u after s steps}\right) \PP\left( \text{u $\mapsto$ v after k steps without attain u}\right) \cdot \beta(s)
%     \\
%     =\ & \sum_{t=1}^{T} \sum_{s + k = t} (W^{s})_{uu} \cdot \left( \sum_{u_{l} \neq u} W_{u u_1} W_{u_1 u_2} \cdots W_{u_{k-1} v} \right)  \cdot \beta(s)
% \end{align*}
